# Supplementary material for: CEFHRI: A Communication Efficient Federated Learning Framework for Recognizing Industrial Human-Robot Interaction
Source: arXiv:2308.14965 source file (2023-08-29)
Supplement: Supplementary file 1 [file appendix.tex]

For each method and dataset, the optimal learning rates for our experiments are mentioned in Table~\ref{tab:lr}. The fine-tuning details are explained in Table~\ref{tab:training_Settings}.
 For the CEFHRI, the bases of the newly added modules are configured with zero initialization. For the additional network, the down-projection layers are initialized with Kaiming Normal ~\cite{he_deep_2016}, while the weights of the up-projection layers are initialized with zero as in \cite{chen_adaptformer_2022}. For prompt tuning, the number of introduced tokens is set to 8 based on optimal performance. For the adapter, we set $\gamma = 0.1$, as in \cite{chen_adaptformer_2022}, while for our designed FLAR-ST-Adapter, we set $\gamma = 1$. The bottleneck dimension, $\hat{d}=64$ in our default settings for the adapters. Any modification to the default settings will be clearly stated.
